# Supplementary material for: Data-Driven Predictive Control for Linear Parameter-Varying Systems
Source: arXiv:2103.16160 source file (2022-01-24)
Supplement: Supplementary file 1 [file appendix.tex]

\appendix
\section{First Appendix}
% remove or comment these lines to remove the appendix (if not necessary)
